# Supplementary material for: Stress effects on vibrational spectra of a cubic hybrid perovskite: A probe of local strain
Source: arXiv:1907.03673 ancillary file (2020-11-21)

Supplementary information for

# Stress Effects on Vibrational Spectra of a Cubic Hybrid Perovskite: A Probe of Local Strain

Kuntal Talit and David A. Strubbe
Department of Physics, University of California, Merced, California 95343

**Table S1:** Relaxed structure parameters for cubic $CH_3NH_3PbI_3$ using different functionals. Lattice parameters and bond lengths in Å and angles in degrees.

| | a | b | c | α | β | γ | Pb-I bond | Pb-I-Pb angle | C-H | N-H | C-N |
|---|---|---|---|---|---|---|---|---|---|---|---|
| **Initial Structure** | 6.288 | 6.228 | 6.374 | 90.003 | 88.744 | 89.986 | 3.250<br>3.078<br>3.215<br>3.174<br>3.140 | 165.151<br>167.237<br>172.011 | 1.099<br>1.100<br>1.100 | 1.047<br>1.047<br>1.042 | 1.481 |
| **Functional** | | | | | | | | | | | |
| LDA | 6.163 | 6.115 | 6.267 | 90.004 | 88.803 | 89.998 | 3.090<br>3.120<br>3.173<br>3.156<br>3.090<br>3.046 | 163.458<br>164.652<br>173.920 | 1.101<br>1.101<br>1.100 | 1.048<br>1.048<br>1.043 | 1.471 |
| PBE | 6.499 | 6.410 | 6.532 | 90.000 | 88.657 | 90.001 | 3.444<br>3.227<br>3.227<br>3.075<br>3.328<br>3.234 | 166.715<br>169.170<br>171.133 | 1.093<br>1.093<br>1.093 | 1.038<br>1.037<br>1.038 | 1.493 |
| PBEsol | 6.291 | 6.248 | 6.378 | 89.999 | 88.645 | 90.000 | 3.146<br>3.146<br>3.238<br>3.085<br>3.220<br>3.171 | 166.527<br>168.411<br>172.732 | 1.099<br>1.099<br>1.098 | 1.044<br>1.041<br>1.044 | 1.482 |

**Fig. S1.** Bandstructure for cubic $CH_3NH_3PbI_3$ using LDA.

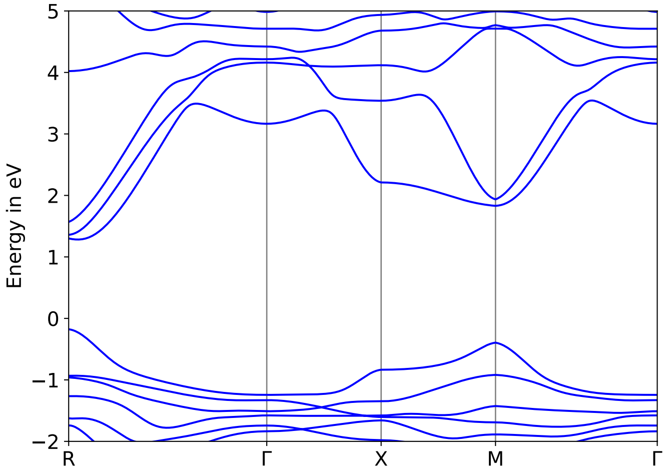

**Table S2:** Bandgap at different k-points using different functionals.

| | Bandgap in eV | |
|---|---|---|
| **Functional Used** | **R** | **M** |
| **LDA** | 1.478 | 2.225 |
| **PBE** | 1.769 | 2.353 |
| **PBEsol** | 1.525 | 2.217 |

**Fig. S2.** Benchmark calculation of the change in optical phonon frequency of c-Si under uniaxial strain along [100], with different DFT functionals. Applied strain breaks the degeneracy of the phonon mode making doubly degenerate (dotted) and singly degenerate (solid) modes.

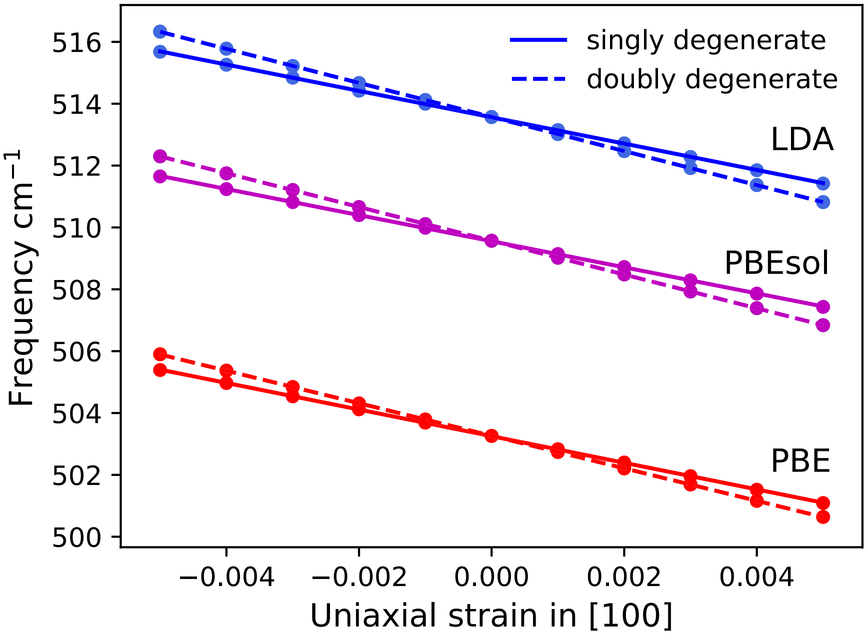


**Table S3:** Benchmark calculation of optical phonon mode frequencies at $q$ = 0 for c-Si, and the split singlet and doublet slopes under uniaxial [100] strain using LDA, PBE and PBEsol. Calculated values are compared with published theoretical and experimental results. LDA has best agreement with experiment.

| Method | lattice constant (Å) | $\omega$ (cm$^{-1}$) | singlet slope (cm$^{-1}$) | doublet slope (cm$^{-1}$) |
|---|---|---|---|---|
| LDA | 5.394 | 514 | -426 | -551 |
| PBE | 5.469 | 503 | -430 | -526 |
| PBEsol | 5.431 | 510 | -422 | -546 |
| LDA[61] | 5.38 | 514 | -424 | -547 |
| Exp't | - | 520±0.5[84] | -481±20[85] | -601±20[85] |

**Table S4:** Complete phonon mode analysis at *q*=0 for cubic $CH_3NH_3PbI_3$. Here IR intensity is in $(D/Å)^2$/amu units and Raman intensity is in $Å^4$/amu units as given by Quantum ESPRESSO. $\Delta\omega$ denotes change in frequency due to rotation of the $CH_3NH_3$ cation inside the Pb-I cage. Raman shift pattern includes all three directions [100], [010], and [001].

| Mode | Freq ($cm^{-1}$) | IR intensity | Raman intensity | Depol. ratio | $CH_3NH_3$ vibration | Pb-I cage vibration | Slope [100] | Slope [010] | Slope [001] | Raman shift pattern | $\Delta\omega$ |
|---|---|---|---|---|---|---|---|---|---|---|---|
| 4 | 20 | 0.19 | 15.25 | 0.75 | translation | Pb-I-Pb bending | 22.50 | -323.83 | 129.83 | linear | 1.66 |
| 5 | 27.97 | 0.16 | 303.36 | 0.15 | libration | Pb-I-Pb rock | -108.00 | -141.33 | 215.83 | parabolic, mixed | 2.19 |
| 6 | 28.3 | 0.42 | 133.24 | 0.32 | libration, translation | Pb-I-Pb bend | 44.50 | 109.33 | -63.00 | parabolic, mixed | -1.06 |
| 7 | 34 | 0.22 | 22.73 | 0.74 | translation | Pb-I-Pb rock | 42.50 | -121.50 | 125.33 | linear | 1.26 |
| 8 | 34.92 | 0.10 | 142.34 | 0.13 | translation | Pb-I-Pb rock | -92.00 | -104.50 | 28.50 | parabolic, mixed | 1.58 |
| 9 | 35.81 | 0.44 | 438.19 | 0.74 | libration, translation | Pb-I-Pb rock | -8.00 | -11.67 | -17.83 | parabolic, mixed | -0.68 |
| 10 | 65.02 | 0.47 | 18.64 | 0.32 | libration<br>asym. bending | no vibration | -203.33 | -449.83 | 204.00 | mixed | 6.15 |
| 11 | 71.65 | 0.87 | 3.42 | 0.75 | libration<br>asym. bending | Pb-I-Pb bending | -352.17 | -263.33 | 42.83 | linear | 5.63 |
| 12 | 85.82 | 4.77 | 193.24 | 0.75 | libration<br>translation | Pb-I-Pb bending<br>Pb-I asym. stretch | -334.83 | -127.83 | -677.00 | linear | 1.51 |
| 13 | 90.4 | 6.13 | 72.27 | 0.58 | libration<br>translation | Pb-I-Pb rock<br>Pb-I stretch | -482.33 | -237.83 | -308.67 | linear | -4.42 |
| 14 | 97.4 | 5.53 | 20.20 | 0.75 | libration<br>spin | Pb-I-Pb bending | -140.83 | -772.67 | -132.83 | linear | 0.43 |
| 15 | 101.37 | 0.46 | 20.37 | 0.26 | translation | Pb-I-Pb rock<br>(only I) | -197.00 | -257.83 | -264.83 | mixed | -3.27 |
| 16 | 128.01 | 0.94 | 28.75 | 0.64 | libration<br>asym. bending | no vibration | -133.33 | -91.33 | 58.17 | mixed | 4.5 |
| 17 | 136.9 | 0.08 | 26.56 | 0.75 | spin | no vibration | -136.50 | 65.83 | 623.50 | mixed | 13.04 |
| 18 | 143.6 | 1.81 | 1.10 | 0.75 | libration<br>asym. bending | no vibration | -164.67 | -394.00 | 161.33 | linear | 3.72 |
| 19 | 312.59 | 0.01 | 38.31 | 0.75 | twist<br>spin | no vibration | 31.00 | 160.00 | 440.00 | linear | 7.13 |
| 20 | 875.68 | 1.39 | 535.87 | 0.75 | asym. bending | no vibration | 34.00 | -23.67 | 166.17 | mixed | 2.19 |
| 21 | 908.09 | 1.57 | 9.96 | 0.75 | asym. bending | no vibration | -20.67 | 103.67 | 123.50 | linear | 2.43 |
| 22 | 1023.57 | 0.25 | 85.70 | 0.45 | sym. bending<br>C-N stretch | no vibration | -25.17 | -52.00 | 9.67 | mixed | 0.08 |
| 23 | 1208.95 | 0.59 | 629.10 | 0.73 | libration<br>asym. bending | no vibration | 22.67 | -43.83 | 88.17 | linear | 0.98 |
| 24 | 1227.42 | 0.05 | 19.45 | 0.75 | libration<br>asym. bending | no vibration | 6.17 | 123.67 | 83.83 | linear | 1.39 |
| 25 | 1365.29 | 0.53 | 222.70 | 0.72 | C-N stretch<br>C-H sym. bending | no vibration | 85.67 | 84.00 | 34.83 | linear | -0.73 |
| 26 | 1403.54 | 0.94 | 82.24 | 0.75 | C-H, N-H<br>asym. bending | no vibration | -11.50 | 44.17 | 95.83 | linear | 1.86 |
| 27 | 1412.6 | 0.28 | 77.60 | 0.69 | C-H, N-H<br>asym. bending | no vibration | 33.67 | -10.50 | 105.50 | linear | 1.36 |
| 28 | 1457.05 | 5.65 | 138.87 | 0.62 | C-N stretch<br>N-H sym. bending<br>C-H asym. bending | no vibration | 63.17 | 74.83 | 88.50 | linear | 0.01 |
| 29 | 1523.94 | 3.74 | 198.71 | 0.57 | N-H asym. bending<br>C-H asym. bending | no vibration | 56.33 | -87.33 | 72.00 | linear | 0.82 |
| 30 | 1537.41 | 7.48 | 15.64 | 0.75 | C-H, N-H<br>asym. bending | no vibration | 79.17 | 302.33 | 90.50 | linear | 0.43 |
| 31 | 2943.14 | 0.11 | 1603.63 | 0.04 | C-N stretch<br>C-H sym. stretching<br>N-H sym. stretching | no vibration | 103.17 | 77.50 | -29.33 | linear | -2.3 |
| 32 | 3036.04 | 3.48 | 1128.95 | 0.75 | C-H, N-H asym.<br>stretch | no vibration | 140.00 | 172.17 | -76.67 | linear | -3.24 |
| 33 | 3045.84 | 0.40 | 1394.65 | 0.73 | C-H, N-H asym.<br>stretch | no vibration | 61.83 | 88.67 | -57.50 | linear | -1.94 |
| 34 | 3053.38 | 15.10 | 4577.19 | 0.59 | N-H asym. stretch<br>C-H asym. stretch | no vibration | 148.67 | 449.00 | -304.50 | linear | -6.05 |
| 35 | 3058.42 | 44.03 | 668.93 | 0.75 | C-H, N-H<br>asym. stretch | no vibration | 170.83 | 547.67 | -328.50 | linear | -6.43 |
| 36 | 3161.71 | 12.70 | 2757.26 | 0.51 | C-H, N-H<br>asym. stretch<br>large N-H stretch | no vibration | -199.33 | -966.67 | -482.67 | mixed | -4.15 |

**Table S5**: Number of modes falling under different slope patterns for uniaxial strain along [100], [010] and [001].

| slope character | non linear | step linear | linear with kinks | linear | parabolic |
|---|---|---|---|---|---|
| **strain along [100]** | 0 | 0 | 8 | 21 | 4 |
| **strain along [010]** | 4 | 4 | 7 | 17 | 1 |
| **strain along [001]** | 2 | 1 | 9 | 21 | 0 |

**Fig S3**. Pb-I bond length changes in each direction of uniaxial strain.

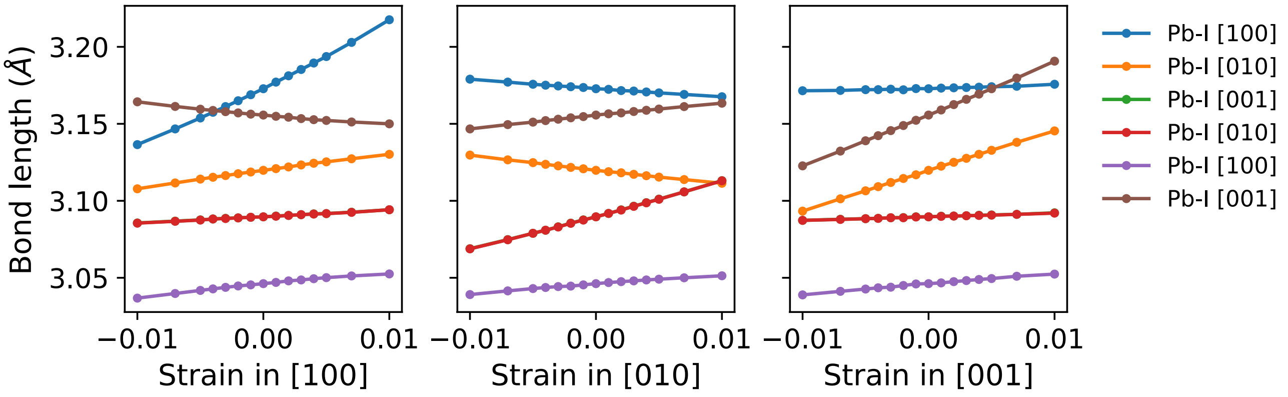


**Fig S4**. Pb-I-Pb bond angle changes due to uniaxial strain.

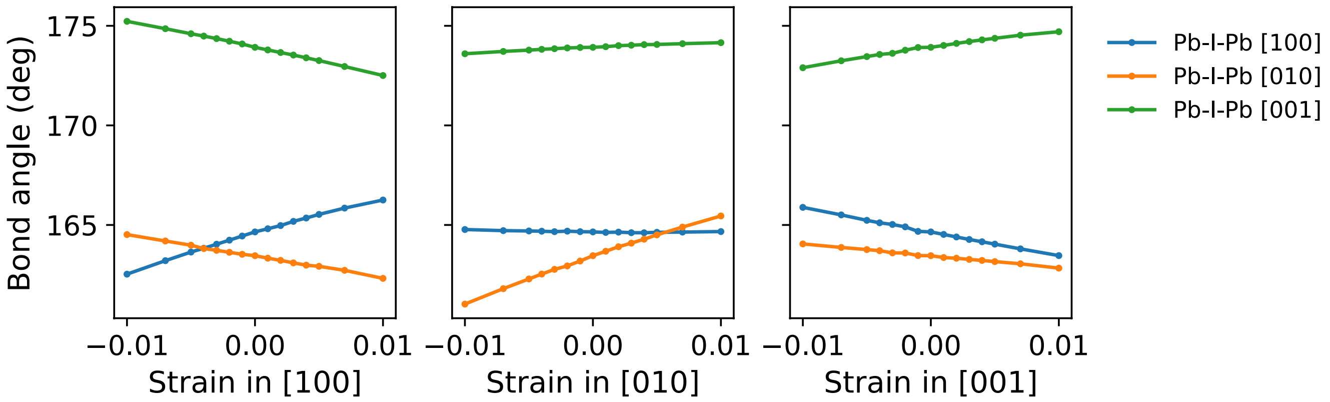

**Fig S5**. C-I distance changes due to uniaxial strain. Iodine atoms are numbered in ascending order of C-I distances.

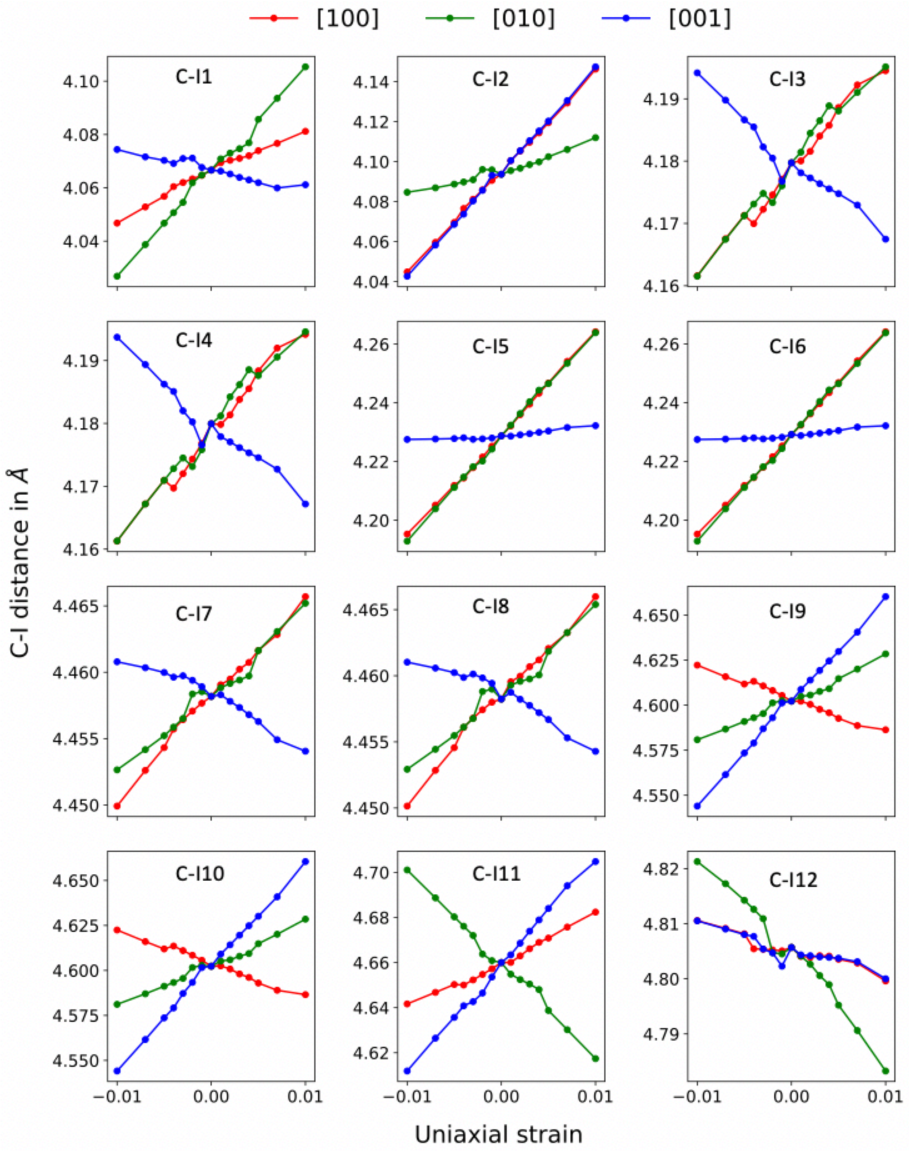


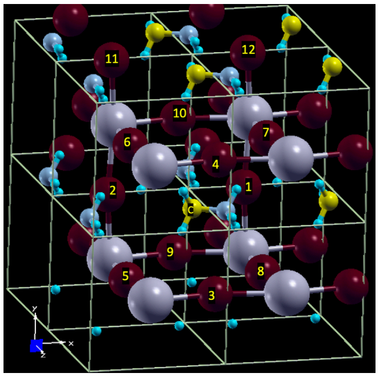


Fig S5a. 2 × 2 × 2 structure of cubic MAPI with numbered iodine atoms.

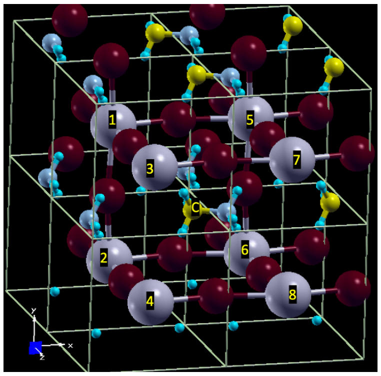


Fig S6a. 2 × 2 × 2 structure of cubic MAPI with numbered lead atoms.

**Fig S6**. C-Pb distance changes due to uniaxial strain. Pb atoms are numbered in ascending order of C-Pb distances.

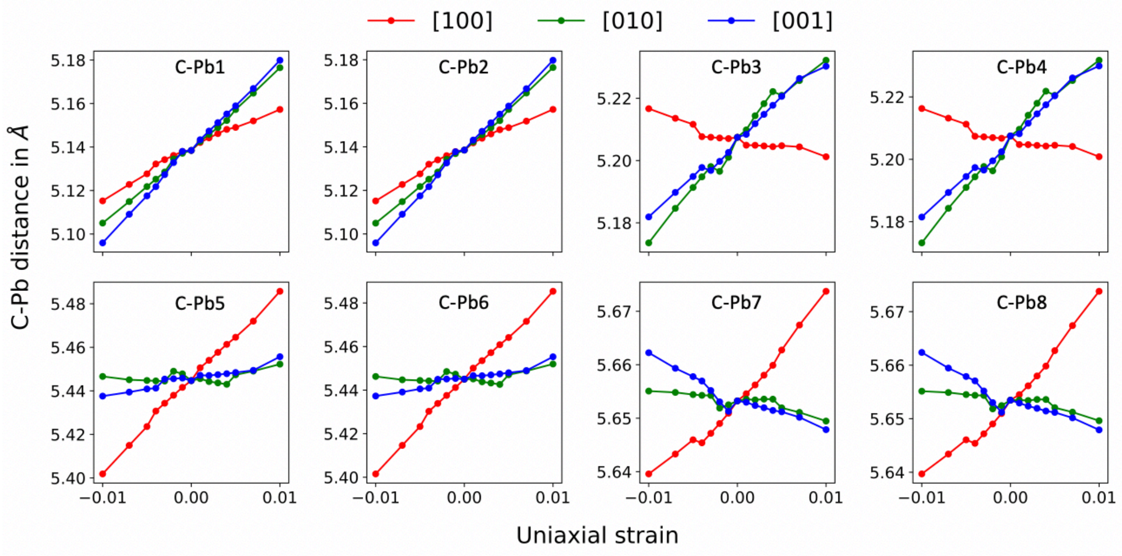

**Fig S7**. N-I distance changes due to uniaxial strain. Iodine atoms are numbered in ascending order of N-I distances.

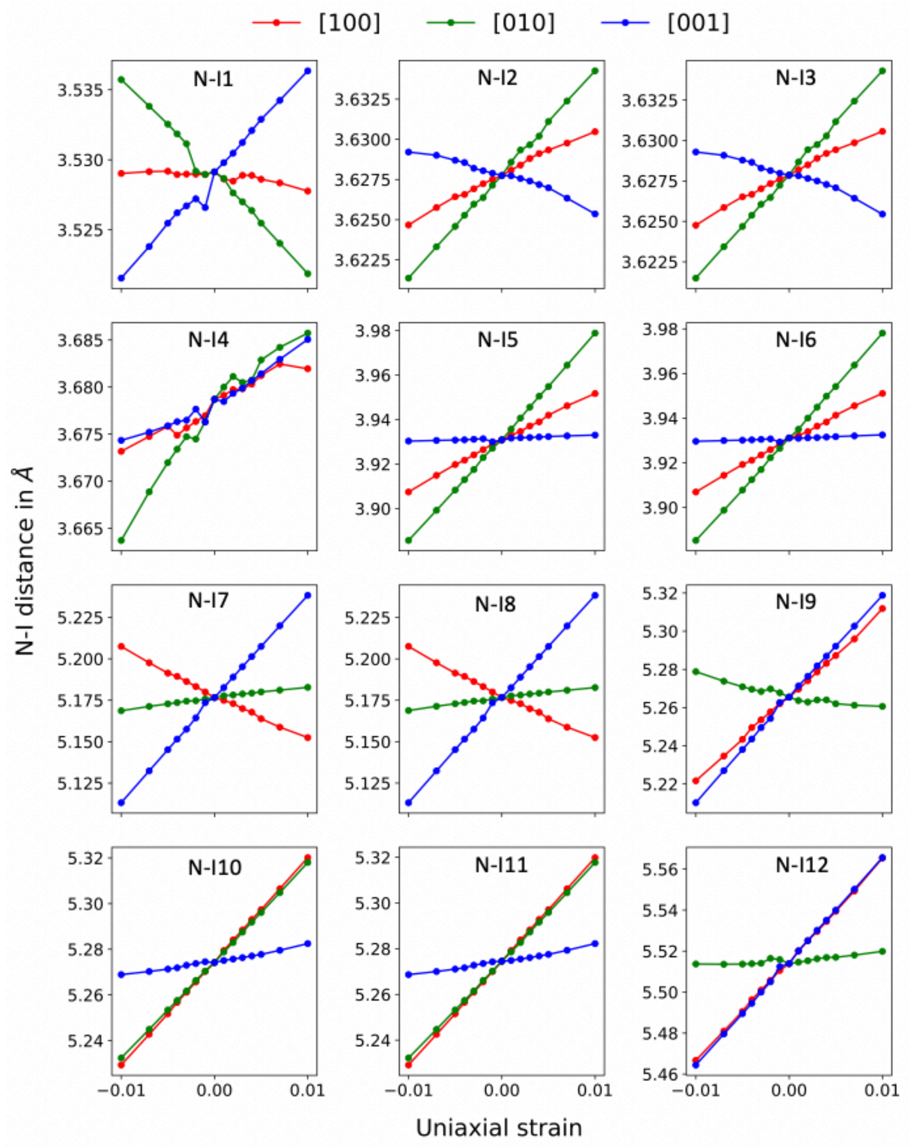


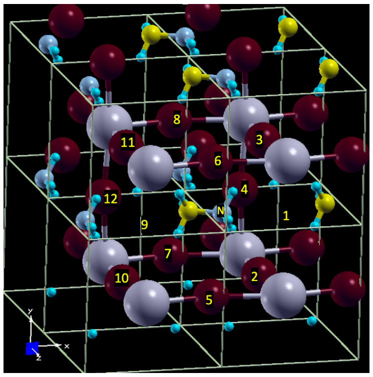


Fig S7a. 2 × 2 × 2 structure of cubic MAPI with numbered lead atoms.

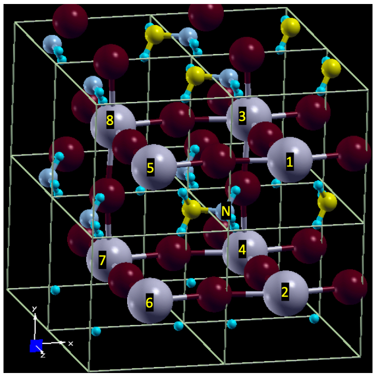


Fig S8a. 2 × 2 × 2 structure of cubic MAPI with numbered lead atoms.

**Fig S8**. N-Pb distance changes due to uniaxial strain. Iodine atoms are numbered in ascending order of N-I distances.

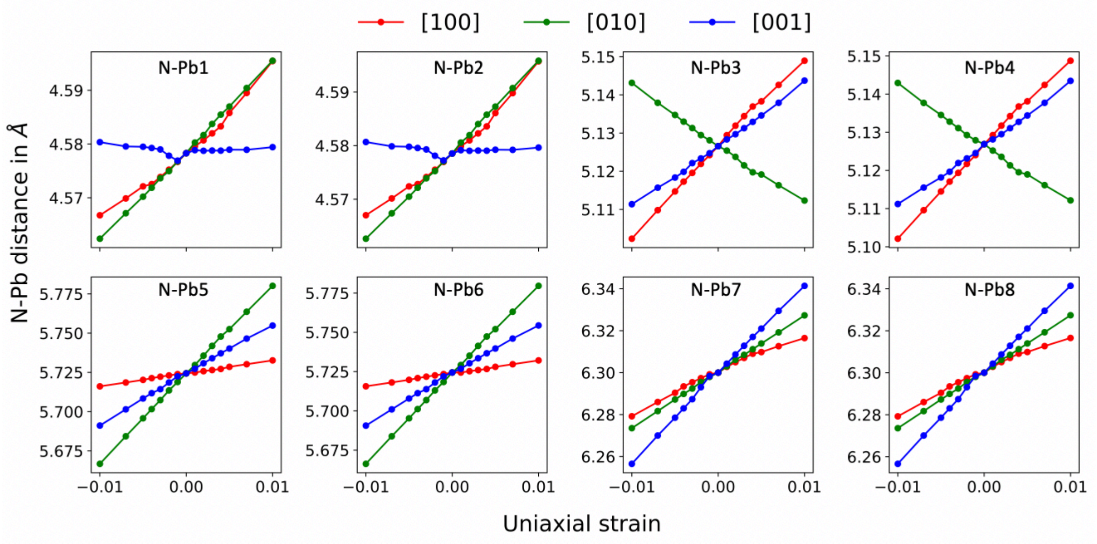

**Fig S9**. Change in N-H bond length due to uniaxial strain.

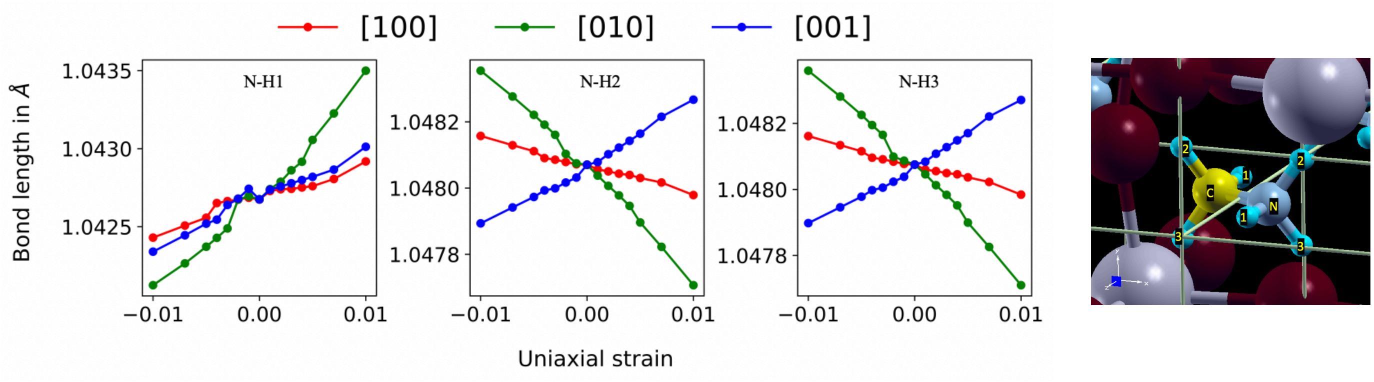


**Fig S10**. Change in C-H bond length due to uniaxial strain.

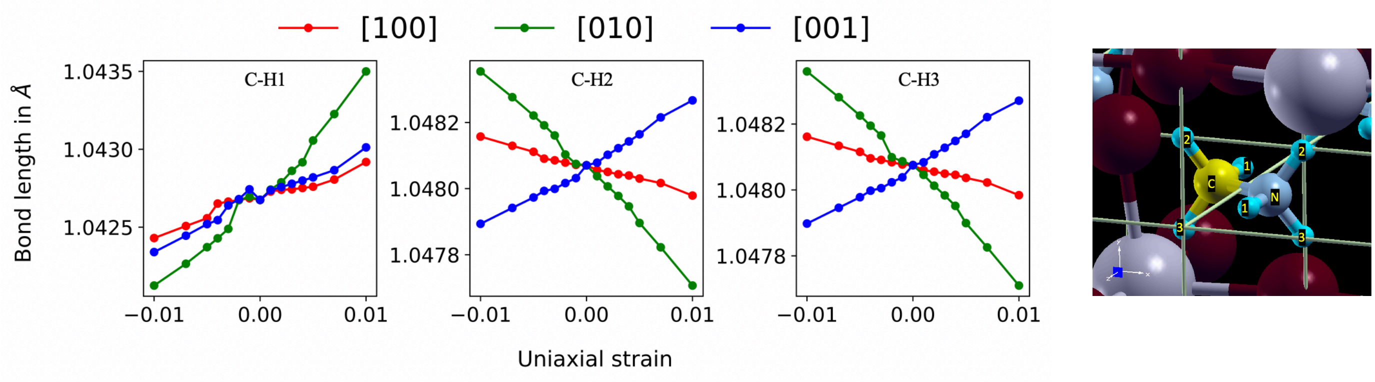


**Fig S11**. Change in orientation of the methylammonium ion. Angle is that between the C-N bond and the *x*-axis, [100] direction.

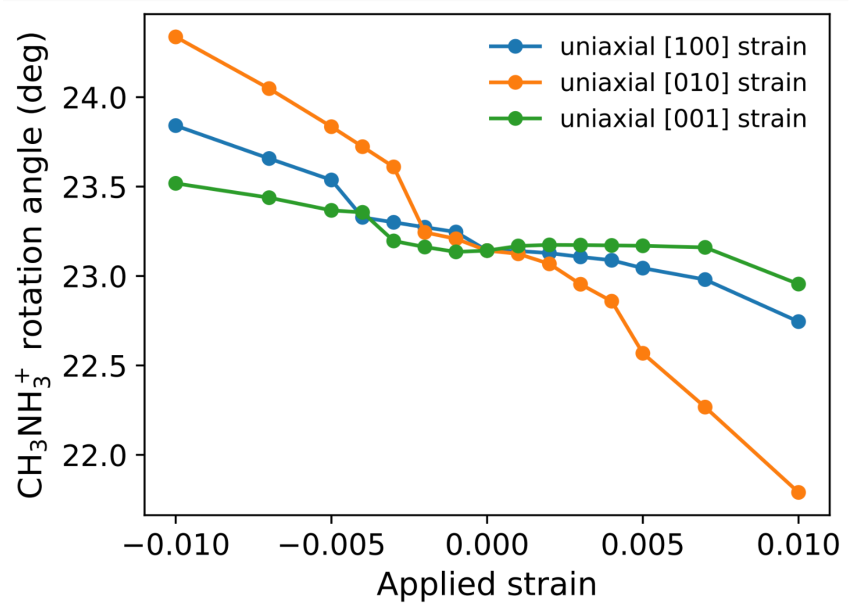

**Fig S12:** Mode eigenvector *vs.* strain, and frequency *vs.* strain, for each of the three crystallographic directions.

---

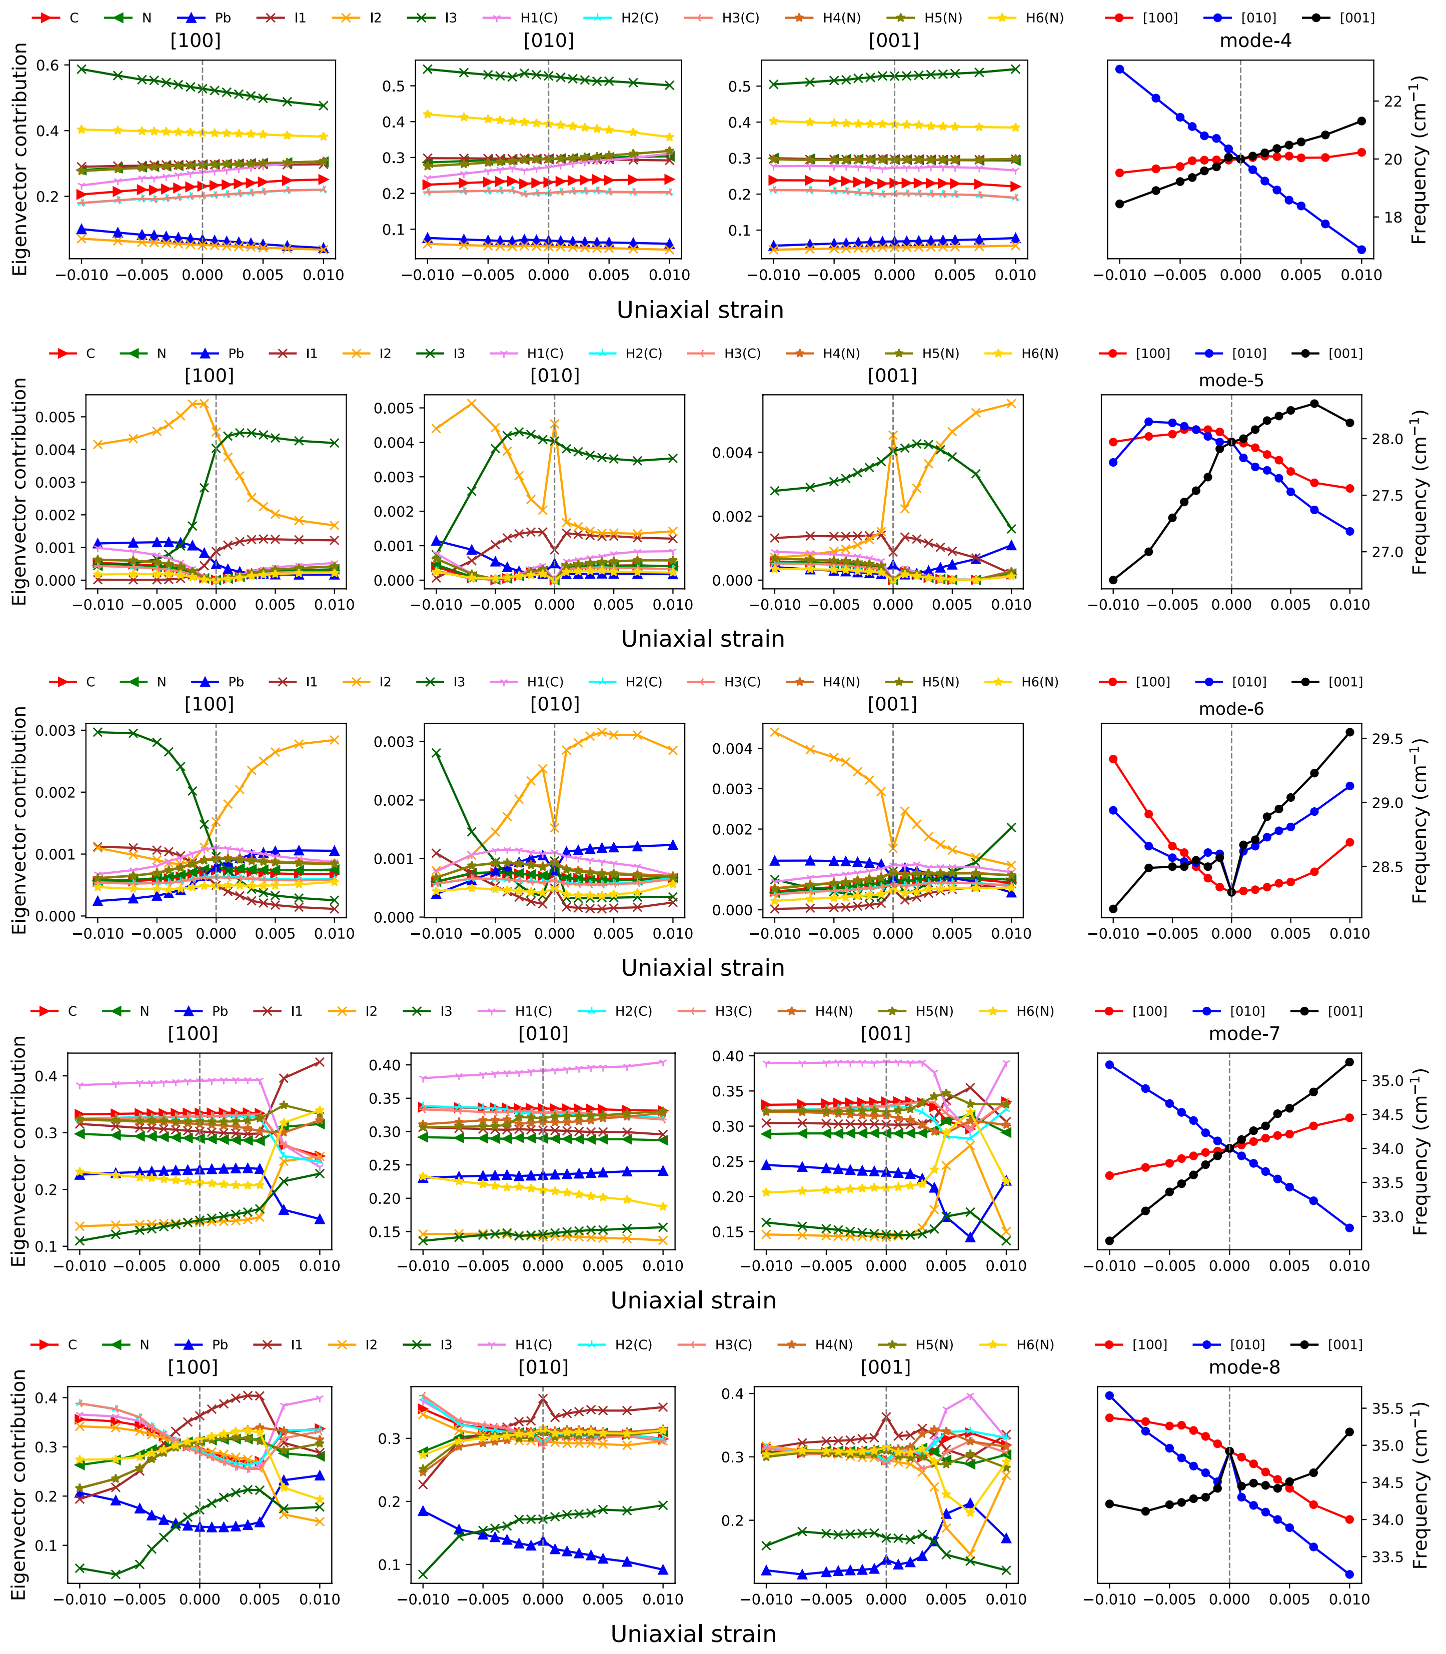

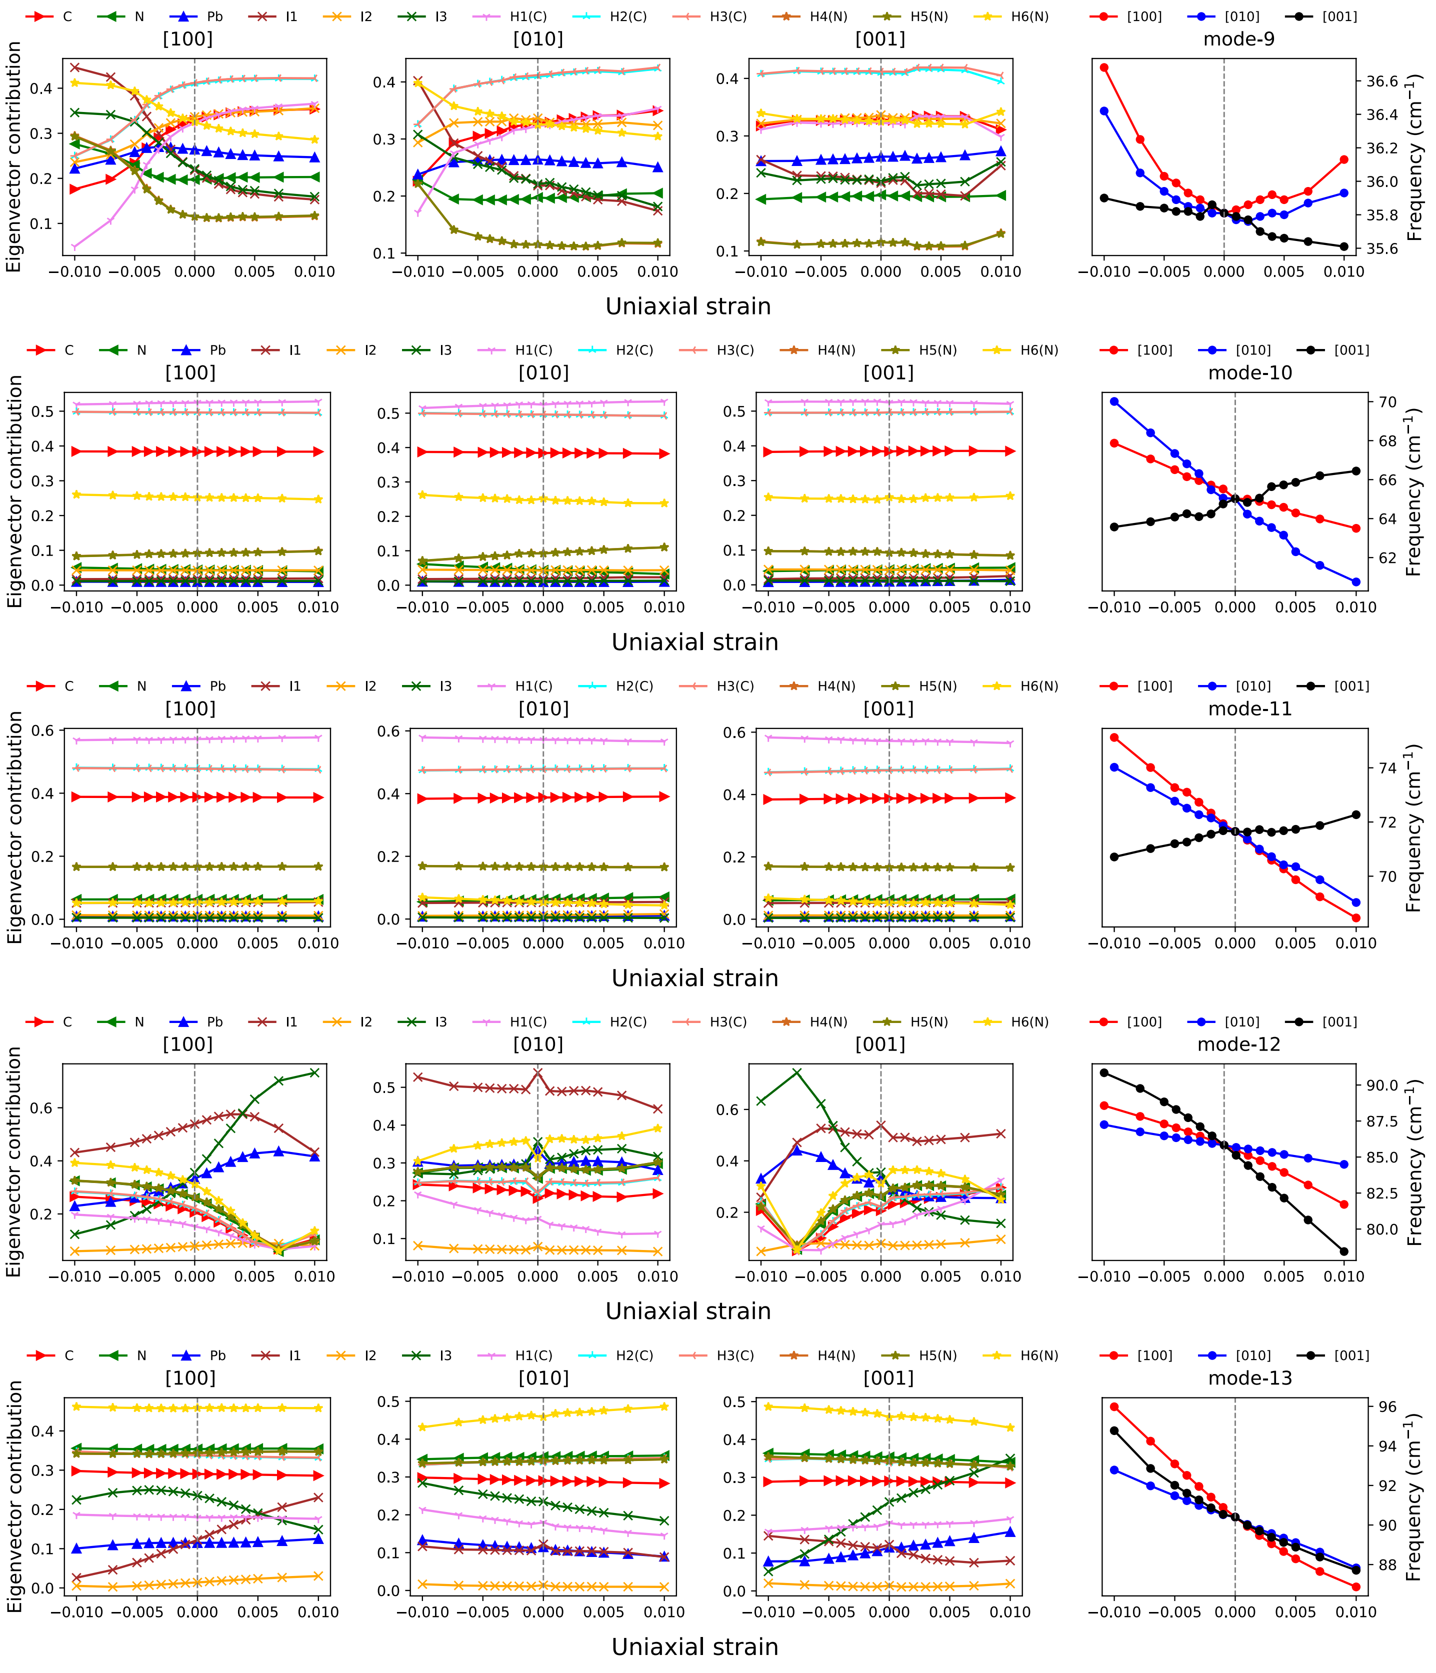
C N Pb I1 I2 I3 H1(C) H2(C) H3(C) H4(N) H5(N) H6(N)
[100] [010] [001]
mode-9
mode-10
mode-11
mode-12
mode-13
Eigenvector contribution
Frequency (cm$^{-1}$)
Uniaxial strain

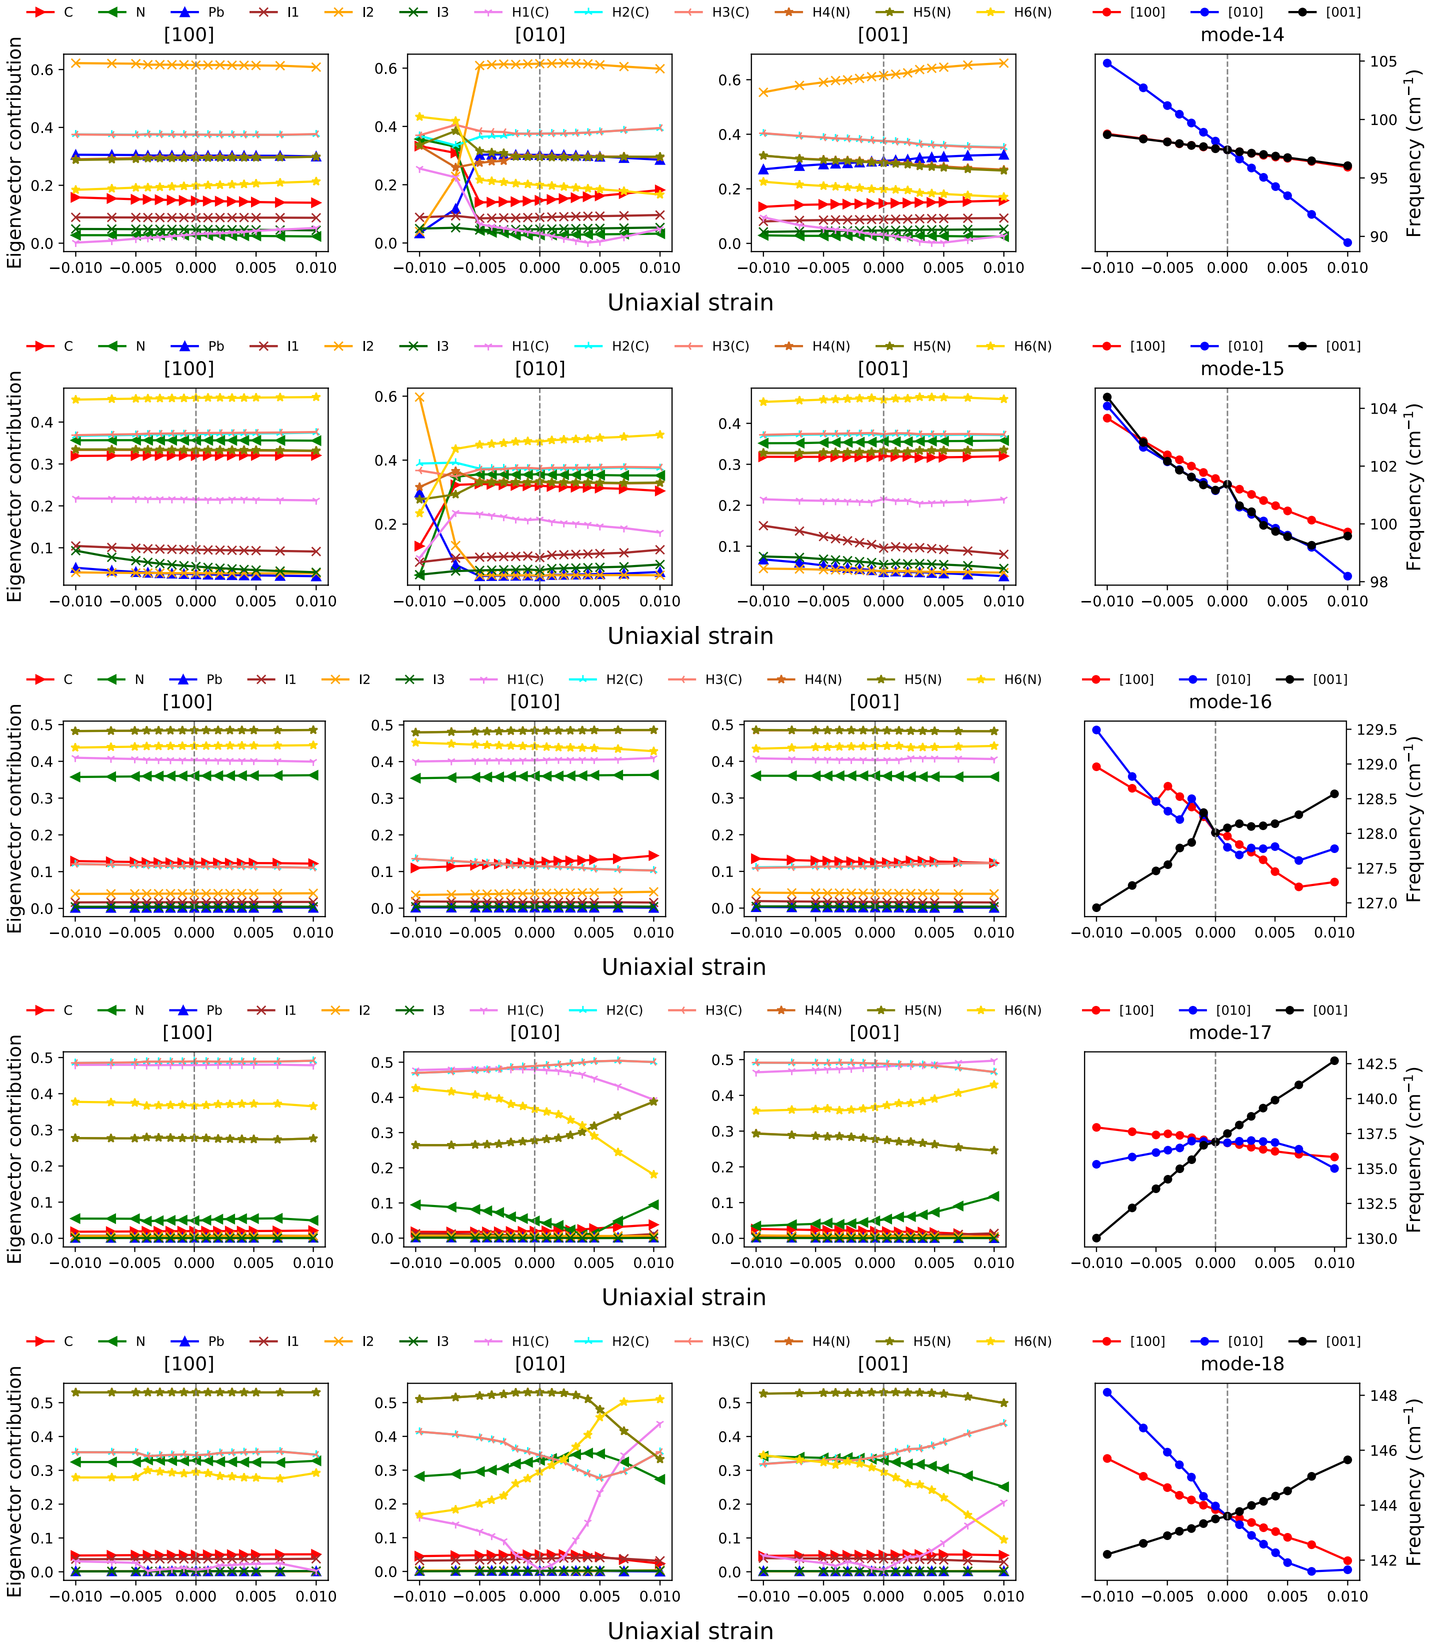

C N Pb I1 I2 I3 H1(C) H2(C) H3(C) H4(N) H5(N) H6(N)
[100] [010] [001]
mode-14
mode-15
mode-16
mode-17
mode-18
Eigenvector contribution
Frequency (cm$^{-1}$)
Uniaxial strain

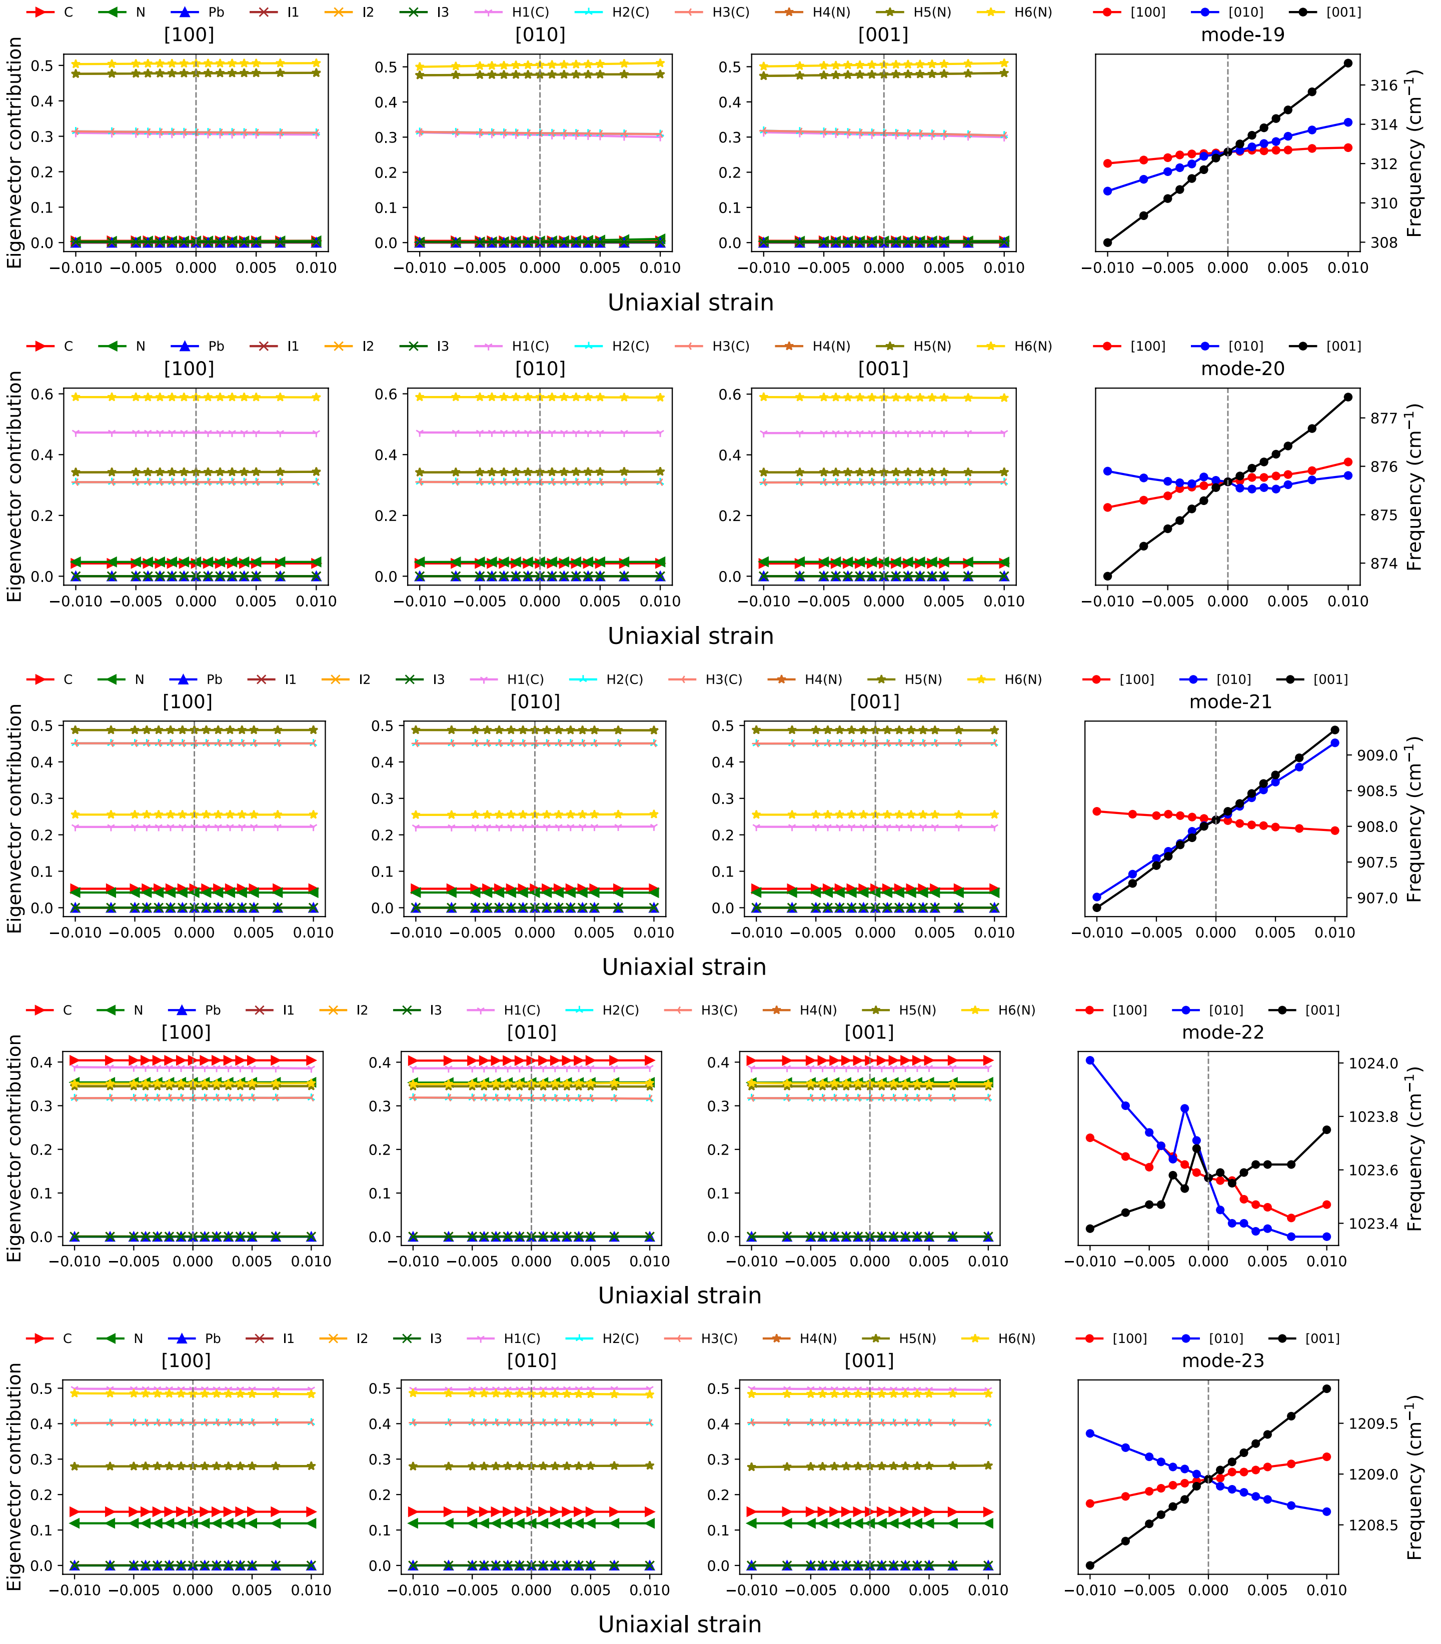
C
N
Pb
I1
I2
I3
H1(C)
H2(C)
H3(C)
H4(N)
H5(N)
H6(N)
[100]
[010]
[001]
mode-19
mode-20
mode-21
mode-22
mode-23
Eigenvector contribution
Frequency (cm$^{-1}$)
Uniaxial strain

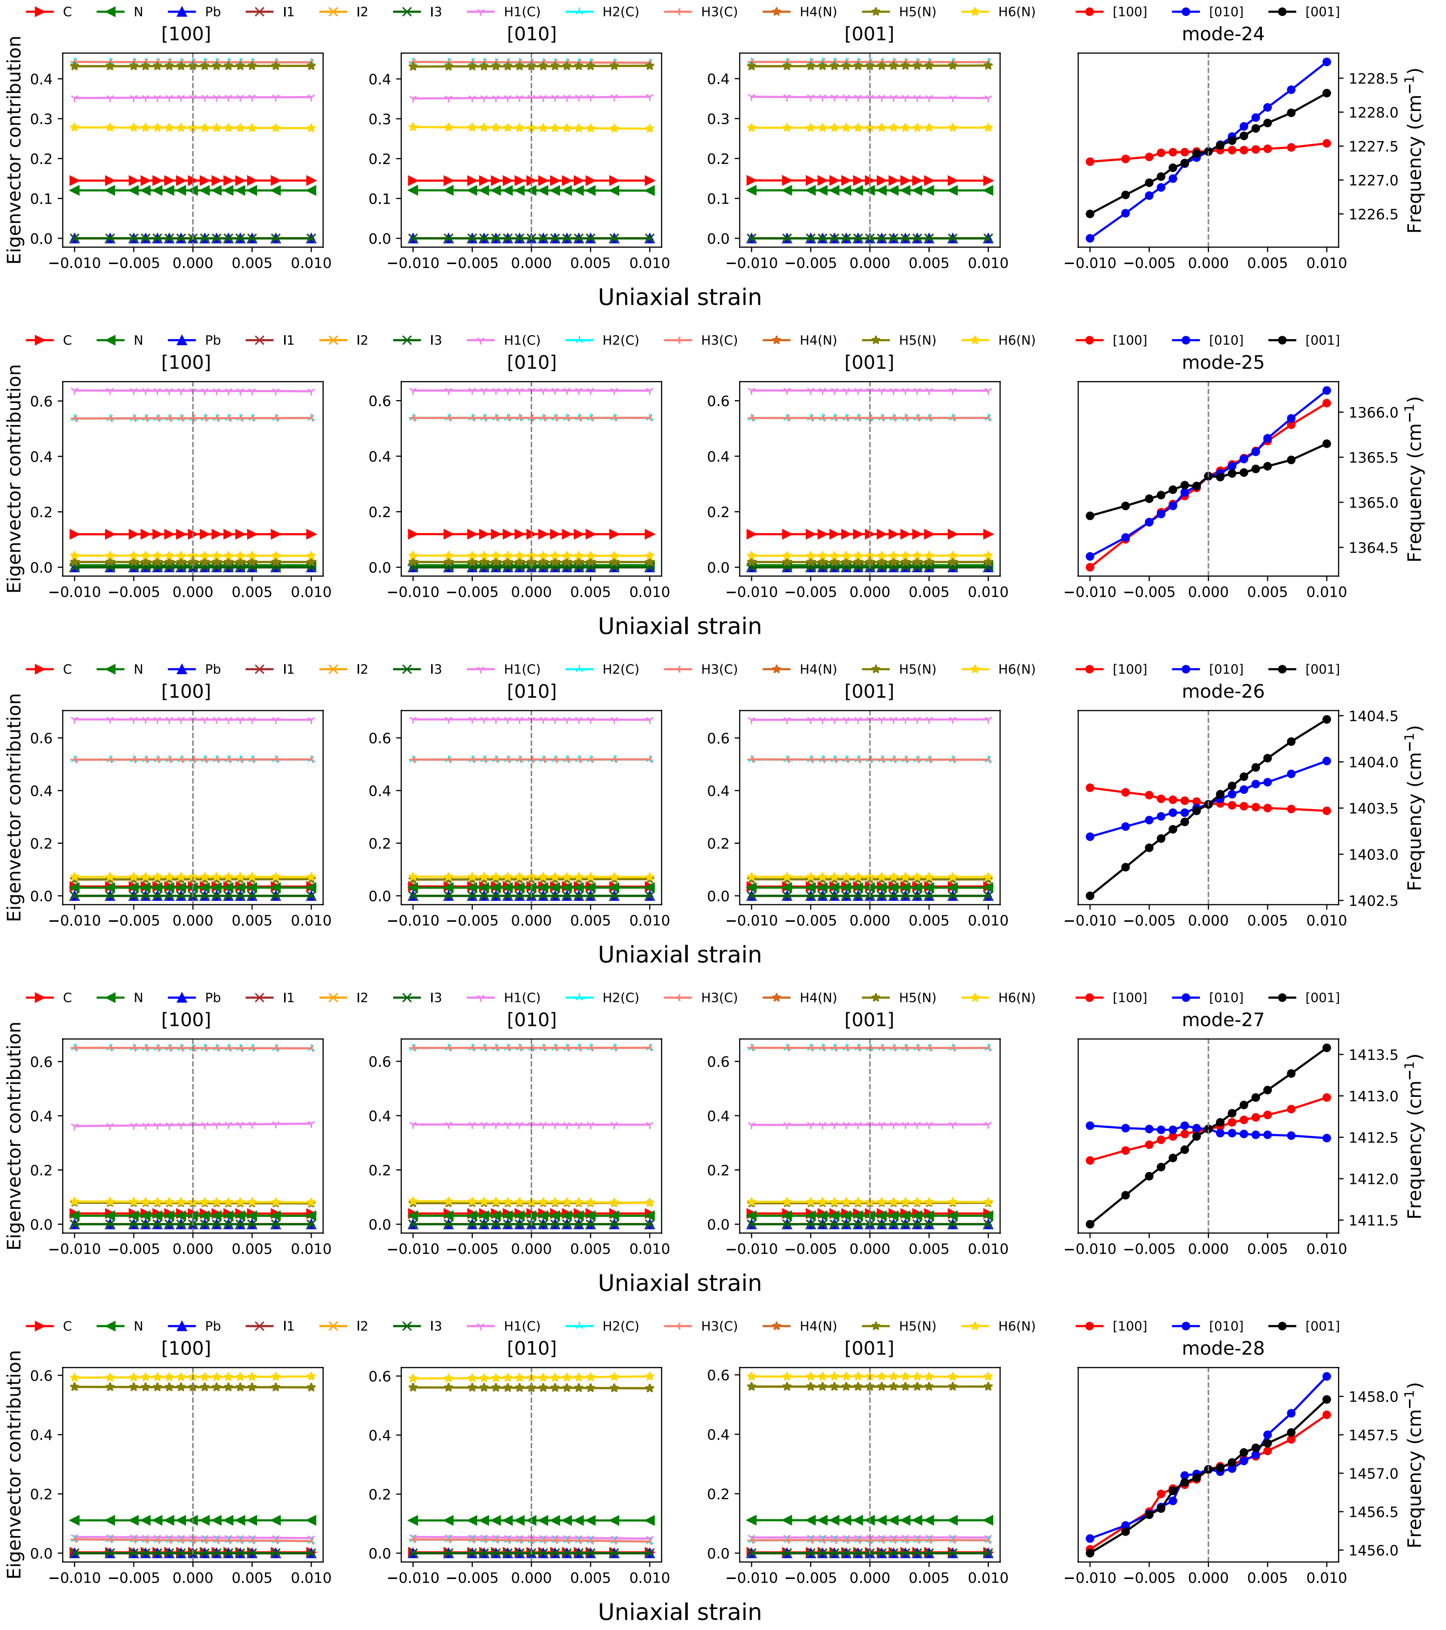
C
N
Pb
I1
I2
I3
H1(C)
H2(C)
H3(C)
H4(N)
H5(N)
H6(N)
[100]
[010]
[001]
mode-24
mode-25
mode-26
mode-27
mode-28
Eigenvector contribution
Uniaxial strain
Frequency (cm$^{-1}$)

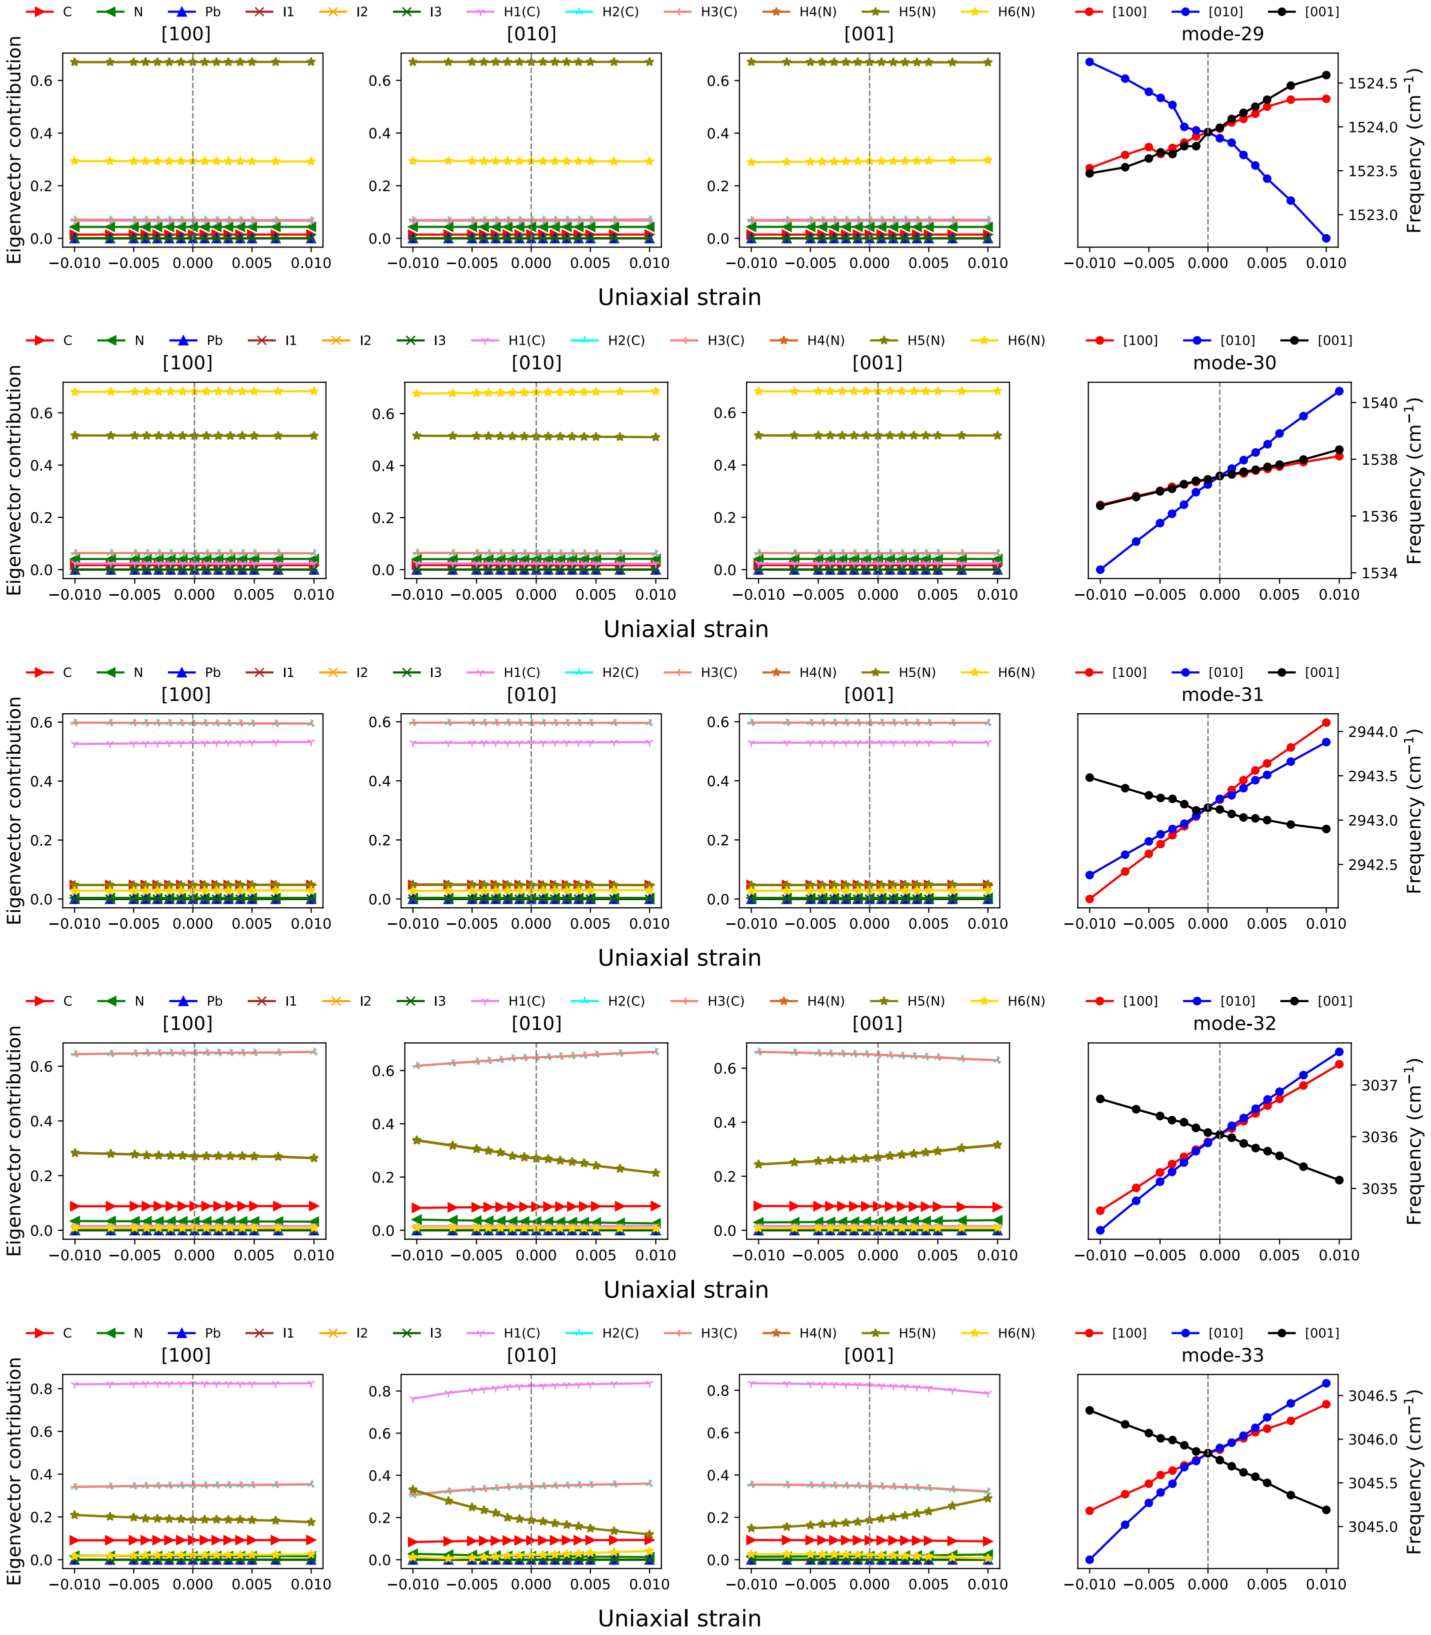
C
N
Pb
I1
I2
I3
H1(C)
H2(C)
H3(C)
H4(N)
H5(N)
H6(N)
[100]
[010]
[001]
mode-29
mode-30
mode-31
mode-32
mode-33
Eigenvector contribution
Uniaxial strain
Frequency (cm$^{-1}$)

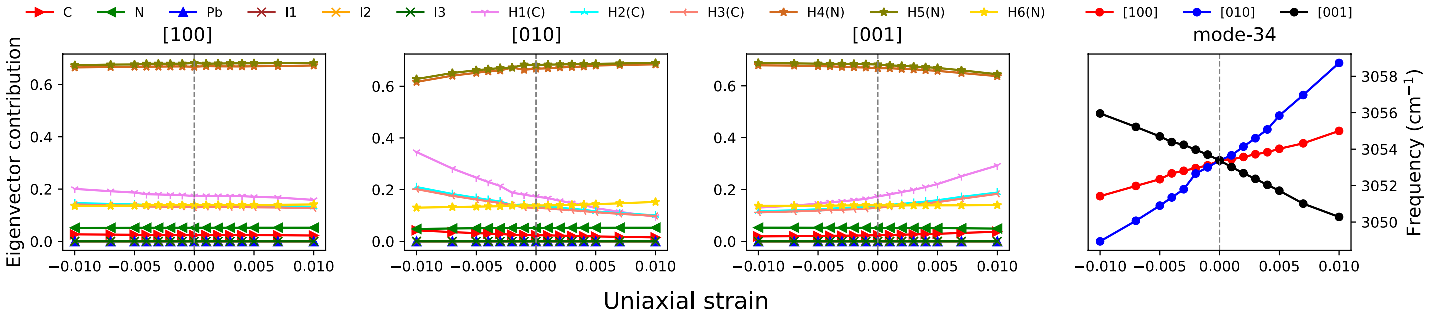


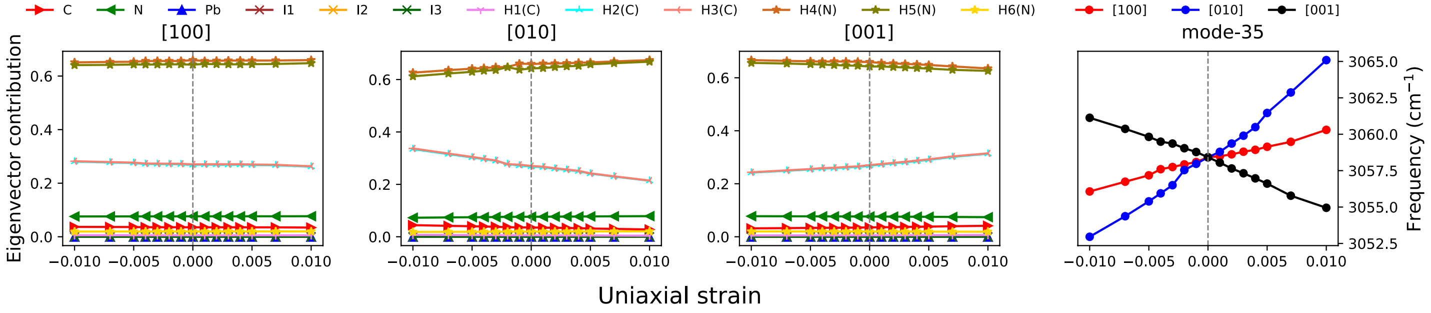


**Fig S13:** Displacement patterns for four most suitable modes to probe local strain with IR/Raman microscopy.

85.82 $cm^{-1}$

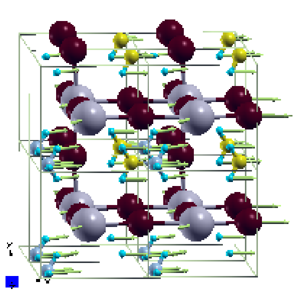

$CH_3NH_3^+$ translation
Pb-I-Pb bend
Pb-I asym. stretch

97.40 $cm^{-1}$

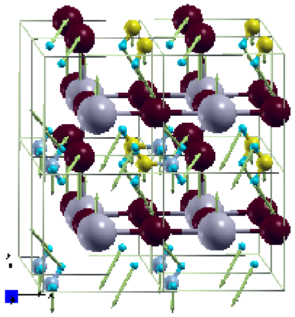

$CH_3NH_3^+$ libration, spin
Pb-I-Pb bend

1457.05 $cm^{-1}$

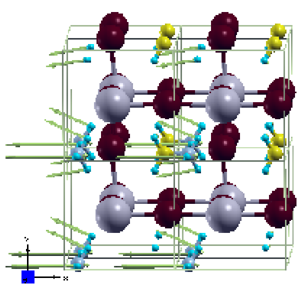

C-N stretch
N-H sym. bend
C-H asym. bend

1537.41 $cm^{-1}$

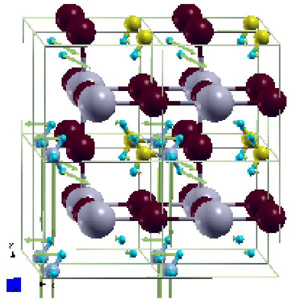

N-H asym. bend
C-H asym. bend

**Table S6**: Comparison of phonon modes at *q*=0, R, and M. Modes at R and M are imaginary at zero strain condition, as well as under compressive and tensile strain at this level.

| Mode No. | *q*=0 zero strain $cm^{-1}$ | *q*=M zero strain $cm^{-1}$ | *q*=R zero strain $cm^{-1}$ | *q*=R comp. strain 0.004 $cm^{-1}$ | *q*=R tensile strain 0.004 $cm^{-1}$ |
|---|---|---|---|---|---|
| 1 | 0.0 | -17.0 | -18.0 | -18.0 | -17.7 |
| 2 | 0.0 | 23.1 | -8.2 | -8.6 | -7.6 |
| 3 | 0.0 | 27.1 | 33.2 | 33.4 | 33.1 |
| 4 | 20.0 | 28.5 | 38.2 | 38.2 | 38.1 |
| 5 | 28.0 | 35.2 | 40.5 | 40.9 | 40.2 |
| 6 | 28.3 | 35.5 | 43.8 | 43.8 | 43.7 |
| 7 | 34.0 | 46.9 | 63.4 | 64.6 | 62.9 |
| 8 | 34.9 | 65.9 | 71.6 | 73.0 | 70.5 |
| 9 | 35.8 | 73.3 | 79.7 | 80.2 | 78.9 |
| 10 | 65.0 | 82.1 | 83.0 | 84.8 | 81.5 |
| 11 | 71.7 | 85.0 | 88.5 | 88.7 | 88.3 |
| 12 | 85.8 | 87.8 | 103.1 | 103.9 | 102.5 |
| 13 | 90.4 | 105.9 | 106.5 | 107.0 | 105.9 |
| 14 | 97.4 | 117.9 | 117.2 | 118.3 | 116.1 |
| 15 | 101.4 | 124.9 | 127.2 | 127.8 | 126.7 |
| 16 | 128.0 | 126.7 | 128.3 | 129.1 | 127.6 |
| 17 | 136.9 | 138.2 | 140.6 | 141.1 | 140.0 |
| 18 | 143.6 | 150.3 | 149.4 | 150.1 | 148.9 |
| 19 | 312.6 | 315.7 | 313.5 | 313.3 | 313.6 |
| 20 | 875.7 | 877.5 | 872.0 | 871.9 | 872.1 |
| 21 | 908.1 | 911.5 | 909.4 | 909.4 | 909.4 |
| 22 | 1023.6 | 1022.9 | 1023.6 | 1023.7 | 1023.4 |
| 23 | 1209.0 | 1205.6 | 1205.9 | 1205.8 | 1206.0 |
| 24 | 1227.4 | 1232.1 | 1232.5 | 1232.5 | 1232.4 |
| 25 | 1365.3 | 1363.0 | 1365.1 | 1364.7 | 1365.3 |
| 26 | 1403.5 | 1403.7 | 1405.8 | 1405.8 | 1405.8 |
| 27 | 1412.6 | 1411.1 | 1412.1 | 1412.0 | 1412.2 |
| 28 | 1457.1 | 1454.7 | 1458.1 | 1457.9 | 1458.2 |
| 29 | 1523.9 | 1520.8 | 1525.5 | 1525.3 | 1525.7 |
| 30 | 1537.4 | 1540.0 | 1541.7 | 1541.4 | 1542.0 |
| 31 | 2943.1 | 2942.9 | 2942.9 | 2942.5 | 2943.4 |
| 32 | 3036.0 | 3038.5 | 3038.5 | 3038.0 | 3039.0 |
| 33 | 3045.8 | 3042.6 | 3042.0 | 3041.4 | 3042.3 |
| 34 | 3053.4 | 3048.5 | 3048.4 | 3047.9 | 3048.8 |
| 35 | 3058.4 | 3076.5 | 3074.8 | 3074.0 | 3075.2 |
| 36 | 3161.7 | 3161.1 | 3161.1 | 3162.2 | 3160.7 |

**Fig. S14:** Dynamical matrix for strain along [100], [010] and [001] directions. (a) Change for compressive strain ($\epsilon = -0.004$). (b) Dynamical matrix at zero strain. (c) Change for tensile strain ($\epsilon = 0.004$). Symbols in both the axes represent atoms and their coordinates. For example, within H(N) block, H3z denotes the z coordinate of the third H attached to N.

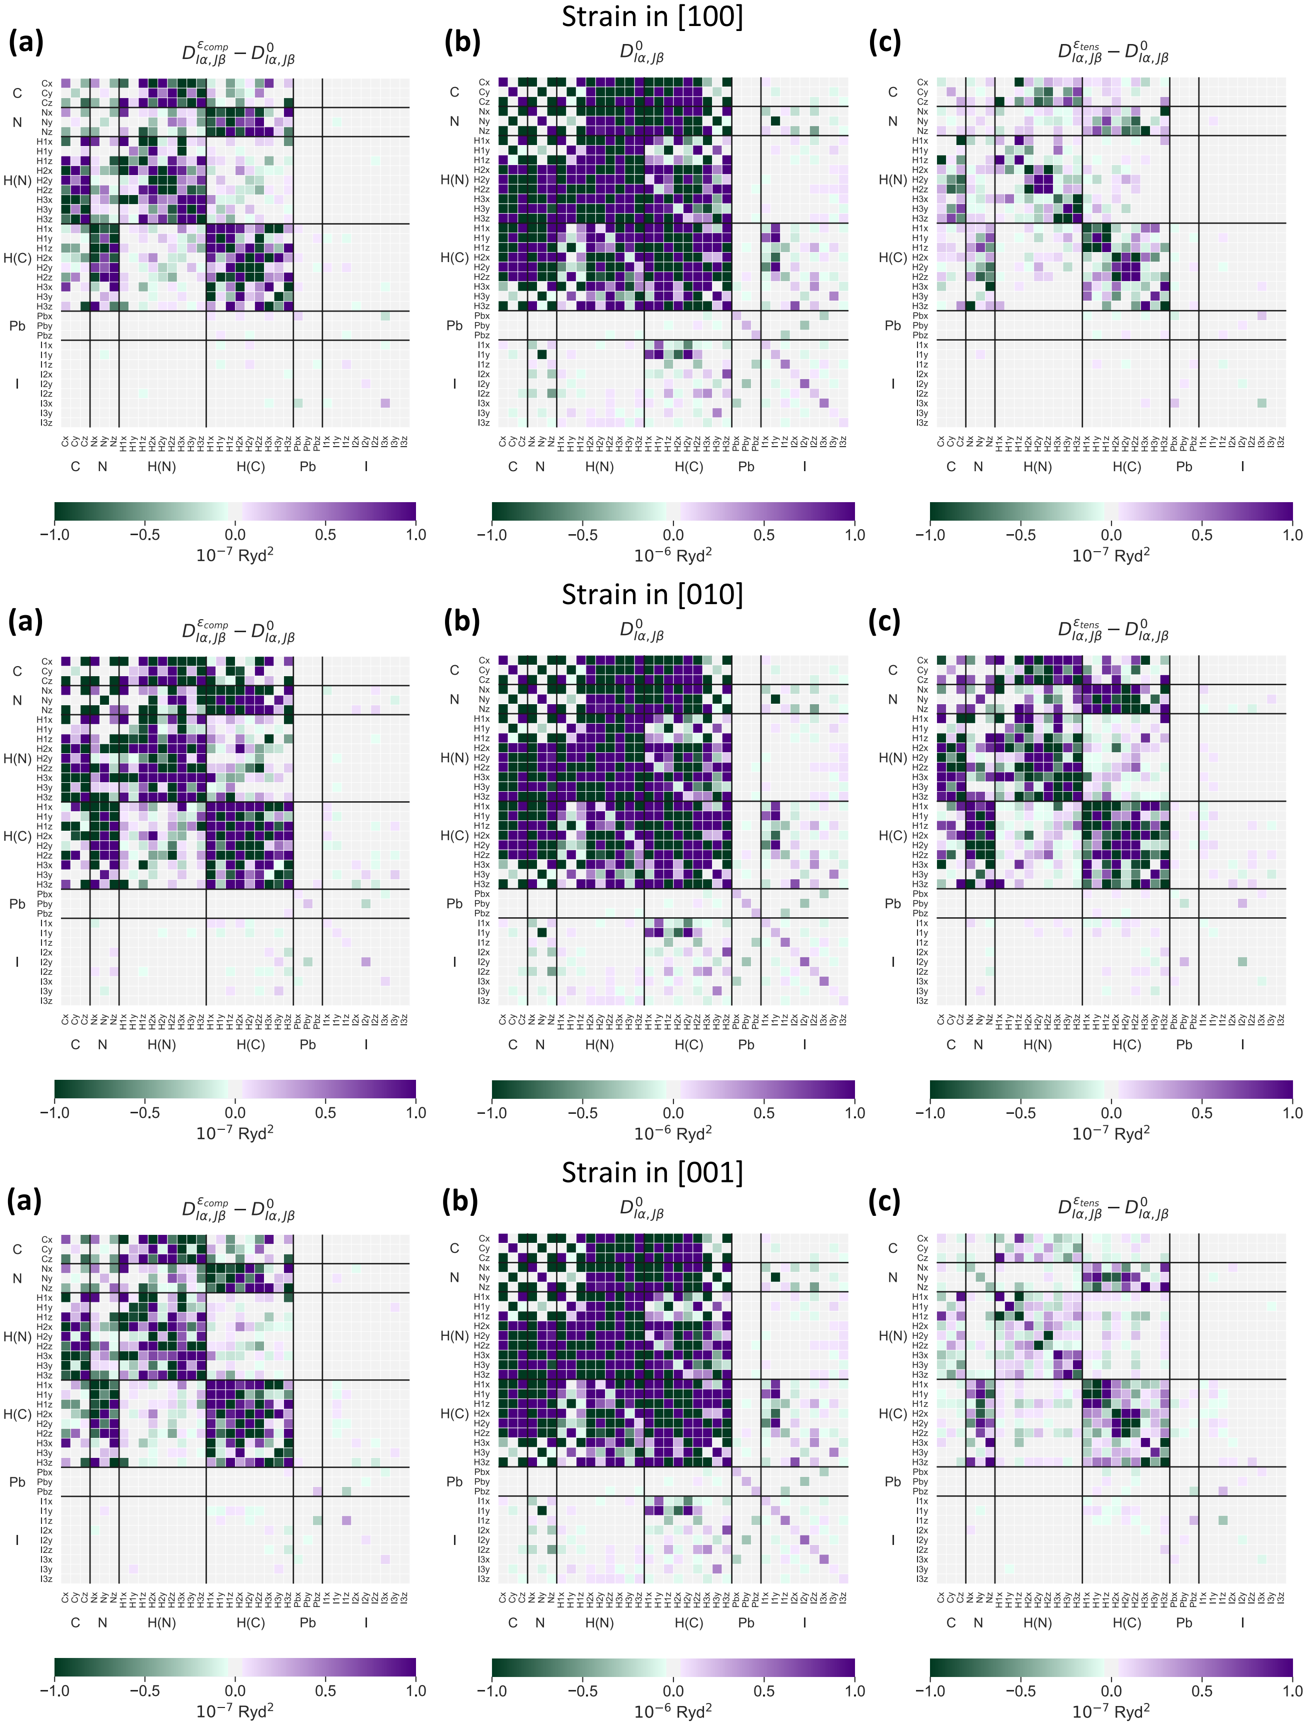

**Fig. S15:** Same as Fig. S11 but with different scales to understand the changes in atomic interaction within the ion itself.

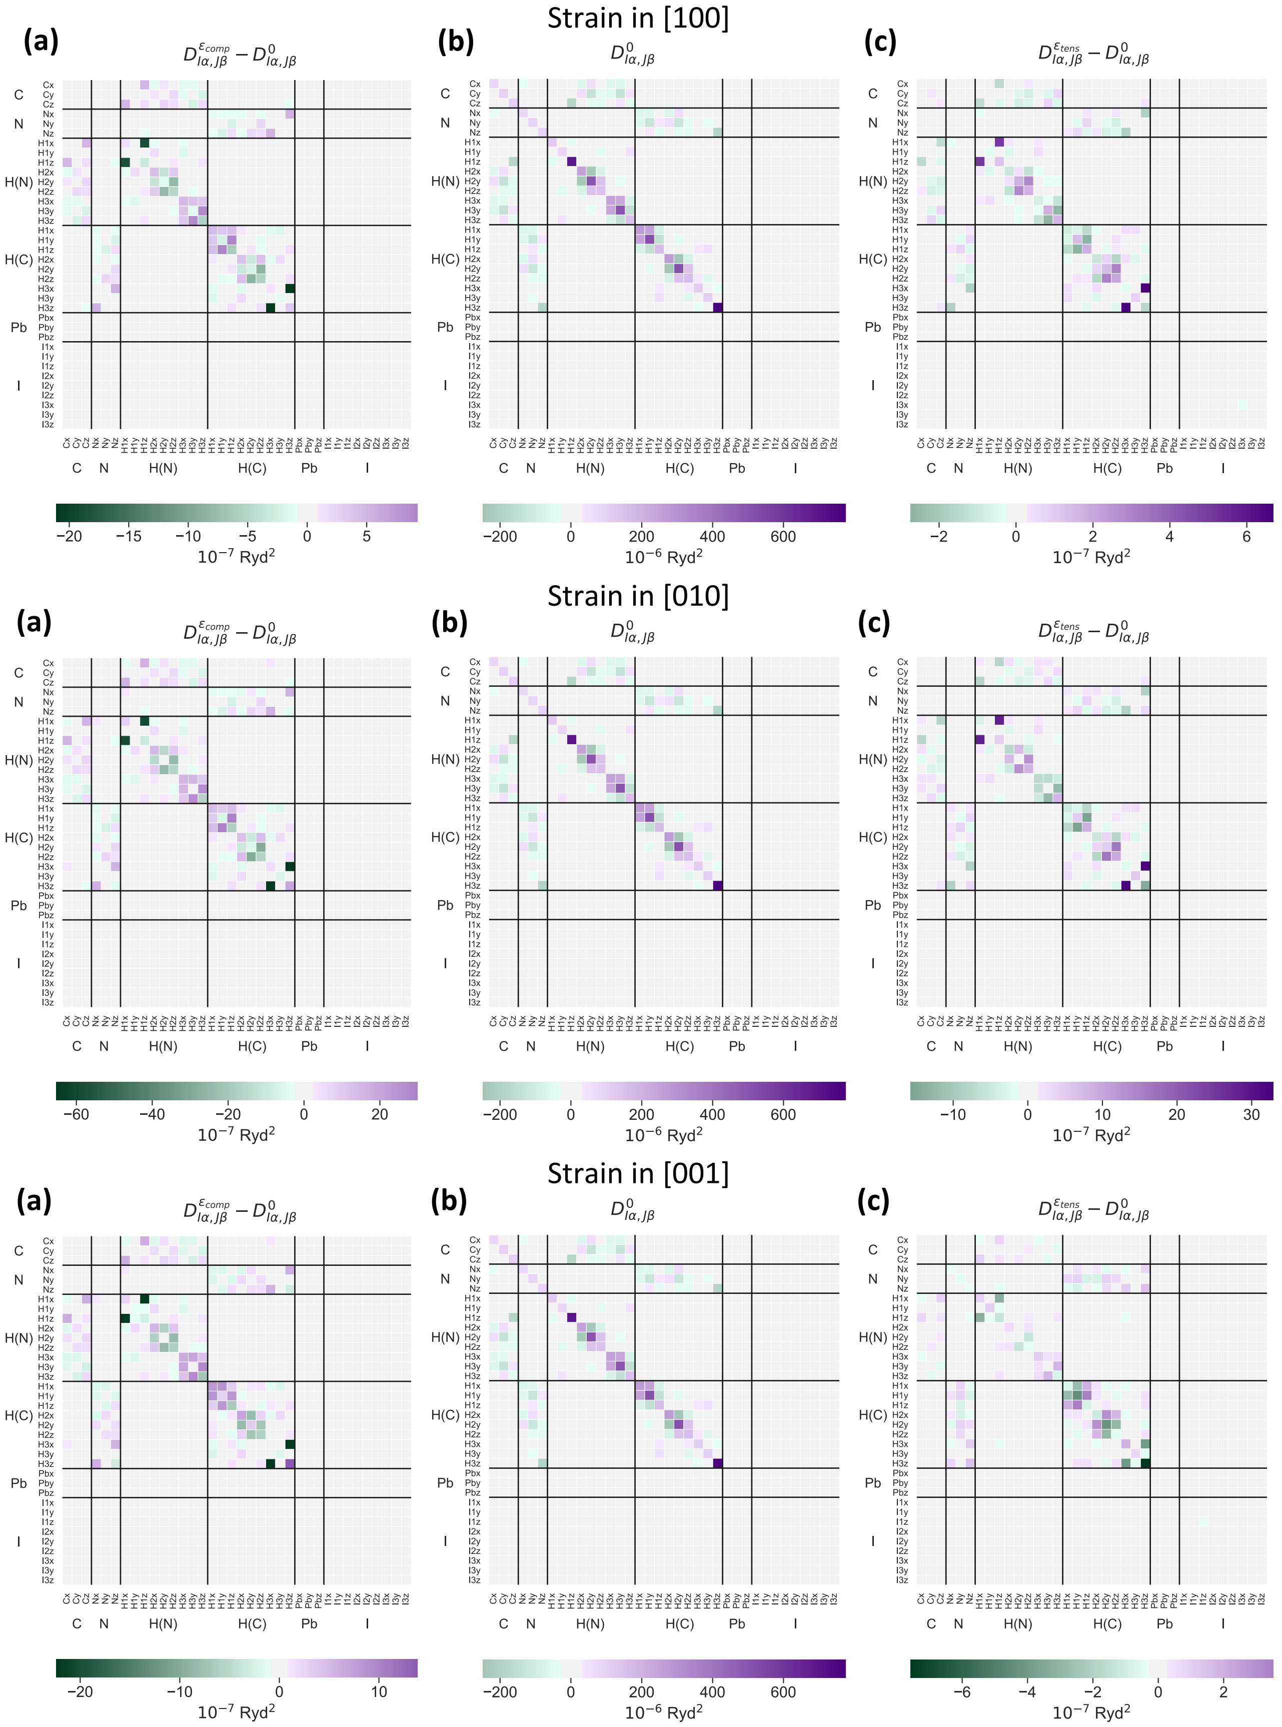

**Fig. S16:** Change of IR intensity with uniaxial strain, for 4 best possible modes for experimental measurement.

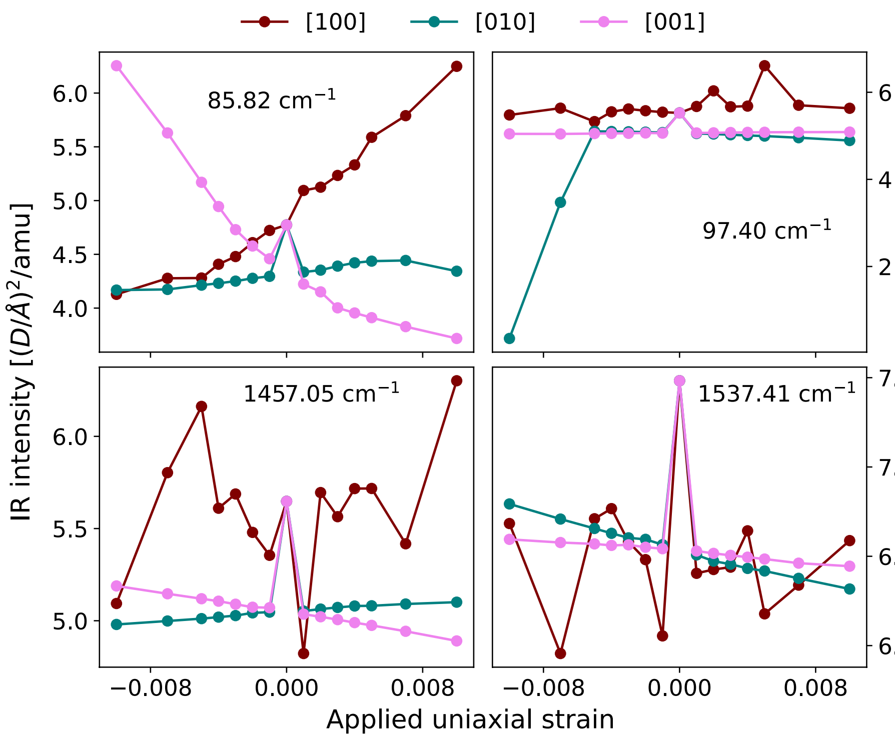


**Fig. S17:** Change of Raman intensity with uniaxial strain for 4 best possible modes for experimental measurement.

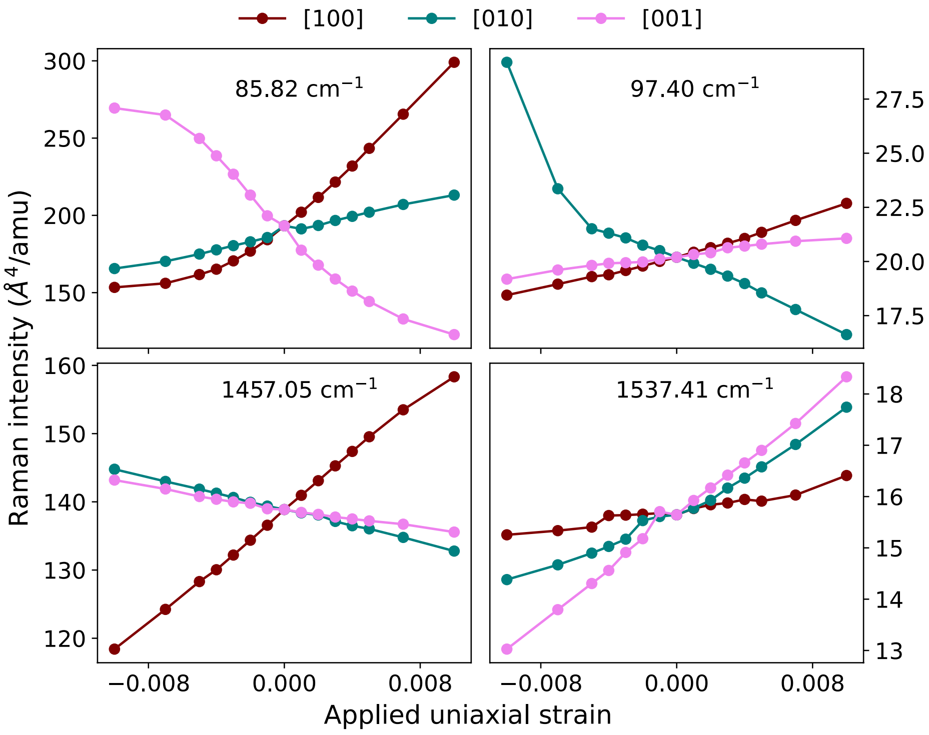

Supplement: Supplementary file 1 [file supplementary.pdf]
